# Supplementary material for: Safety Screening for Voltage Control in Active Distribution Grids via Distributionally Robust Conformal Screening
Source: arXiv:2608.30889 source file (2026-08-31)
Supplement: Supplementary file 1 [file 07_Appendix.tex]

\section{Positioning Relative to Related Assurance Methods}
\label{app:positioning}

Table~\ref{tab:positioning} provides a qualitative positioning of DR-CSS relative to related assurance approaches. The comparison is intended to clarify the scope of the proposed method rather than rank the methods. The selected columns highlight the combination of properties targeted by DR-CSS: feeder-level voltage control, coverage guarantees, robustness to distribution shift, validation of learning-based controllers, and scenario-level accept/warning decisions.

\input{02_related_work_table}


% \section{Controllers used in Experiments}

% We consider two inverter-control configurations, a behavioural droop controller and a target RL controller provided by the MAPDN benchmark~\cite{Wang2021MARLVoltage}.

% \subsubsection{Droop Controller}

% The first controller implements the standard piecewise-linear
% Volt-Var droop characteristic, defined as:
% %
% \begin{equation}
%   U_i(t) =
%   \begin{cases}
%     \bar{q}_i,
%       & V_i(t) \leq V_{\mathrm{db}}^{-}, \\[2pt]
%     -\dfrac{\bar{q}_i}
%       {V_{\mathrm{db}}^{+}-V_{\mathrm{db}}^{-}}
%       \bigl(V_i(t)-V_{\mathrm{db}}^{-}\bigr),
%       & V_{\mathrm{db}}^{-}<V_i(t)<V_{\mathrm{db}}^{+}, \\[4pt]
%     -\bar{q}_i,
%       & V_i(t) \geq V_{\mathrm{db}}^{+}.
%   \end{cases}
%   \label{eq:droop}
% \end{equation}
% %
% The dead-band boundaries are set to
% $V_{\mathrm{db}}^{-}=0.95\,\mathrm{p.u.}$ and
% $V_{\mathrm{db}}^{+}=1.05\,\mathrm{p.u.}$, matching the admissible
% voltage limits. The quantity $ \bar{q}_i=\sqrt{S_i^2-P_i(t)^2}$ denotes the maximum feasible reactive-power magnitude at bus $i$.
% Because the droop law depends only on local measurements, its
% neighborhood is $\mathcal{N}_i=\{i\}$, and no communication between
% agents is required.

% \subsubsection{MARL Controller}

% The second configuration employs the Independent Deep Deterministic
% Policy Gradient (IDDPG) algorithm implemented in the MAPDN
% framework~\cite{Wang2021MARLVoltage}. In this configuration, a single
% inverter $i^{*}\in\mathcal{I}_{\mathrm{inv}}$ is controlled by a trained
% IDDPG actor. The agent observes the voltage magnitudes and active-power
% injections of the inverter buses in its assigned region
% $\mathcal{N}_{i^{*}}$. Based on this observation, it produces the
% continuous reactive-power setpoint
% \[
%     U_{i^{*}}(t)
%     =
%     \pi_{i^{*}}^{\mathrm{RL}}\!\left(o_{i^{*}}(t)\right)
%     \in[-\bar{q}_{i^{*}},\,\bar{q}_{i^{*}}].
% \]
% All other inverter agents continue to follow the droop law in
% \eqref{eq:droop}. The IDDPG agent is trained using the L1-shaped voltage-barrier reward
% introduced in~\cite{Wang2021MARLVoltage}:
% %
% \begin{equation}
%   r(t)
%   =
%   -\frac{1}{|\mathcal{B}|}
%   \sum_{i\in\mathcal{B}} l_v\!\left(V_i(t)\right)
%   -\alpha_{\mathrm{r}}
%   \frac{1}{|\mathcal{I}_{\mathrm{inv}}|}
%   \left\|U(t)\right\|_1,
%   \label{eq:reward}
% \end{equation}
% %
% where $\alpha_{\mathrm{r}}\in(0,1)$ controls the penalty on
% reactive-power usage. We use $\alpha_{\mathrm{r}}$ here to distinguish
% the reward coefficient from the conformal miscoverage level introduced
% later. The voltage-barrier function is
% %
% \begin{equation}
%   l_v\!\left(V_i(t)\right)
%   =
%   \max\!\left(V_{\min}-V_i(t),\,0\right)
%   +
%   \max\!\left(V_i(t)-V_{\max},\,0\right).
%   \label{eq:l1barrier}
% \end{equation}
% %
% This function is zero when the voltage lies within the admissible range
% $[V_{\min},V_{\max}]$ and increases linearly with the magnitude of a
% voltage violation.

% The IDDPG actor and critic networks are trained in the
% PandaPower-based MAPDN simulator using the training scenarios, while
% the droop-controlled agents remain fixed. After training, the resulting
% mixed policy, consisting of one IDDPG agent and
% $|\mathcal{I}_{\mathrm{inv}}|-1$ droop agents, is frozen and treated as
% a black box during calibration and testing.

\subsection{Details on the Robust Statistical Abstraction}
\label{app:robust_calibration_details}

This appendix provides additional explanation of the robust conformal step used in DR-CSS. The goal is to clarify how the nominal simulator is converted into a statistical safety band.

For a scenario \(x\), the simulator returns a single trajectory \(\hat v_{H+1:T}=\Phi_M(x)\). If this trajectory is treated as exact, then the predictive distribution is the point mass \(P_x^{\mathrm{nom}}=\delta_{\hat v_{H+1:T}}\). This means that the simulator assigns probability one to the simulated trajectory and probability zero to all other possible futures. Such a representation is too confident for power-system validation, because the real trajectory may differ from the simulated one due to model mismatch, forecast error, topology uncertainty, measurement error, controller delay, or unmodeled dynamics.

DR-CSS therefore models the simulation error rather than trusting the simulated trajectory directly. For each calibration case, the scalar score
\[
s_j =
\max_{t\in\mathcal T_f}\max_{i\in\mathcal B}
\gamma_t\sigma_i
\left|V_i^j(t)-\hat V_i^j(t)\right|
\]
records the worst voltage prediction error over the whole horizon. This reduces a high-dimensional trajectory error to one safety-relevant number. The empirical distribution
\[
\widehat P_{\mathrm{cal}}^S
=
\frac{1}{n_{\mathrm{cal}}}
\sum_{j=1}^{n_{\mathrm{cal}}}\delta_{s_j}
\]
is therefore a histogram of past worst-case simulation errors.

Standard conformal calibration uses a high quantile of this histogram. For \(\alpha=0.05\), this is approximately the 95\% quantile of the historical worst-case errors. The resulting band is valid when future errors are statistically similar to calibration errors. In conformal prediction, this similarity condition is called exchangeability. In the present setting, it means that future simulation-to-real voltage errors should behave like the historical errors used for calibration.

Controller replacement may violate this condition. Historical data may come from a baseline controller, while the tested deployment uses a new controller. The new controller can move the system into different operating regions and change the simulation-error distribution. DR-CSS accounts for this by considering plausible future score distributions \(Q\) near the calibration score distribution \(\widehat P_{\mathrm{cal}}^S\).

Using total variation, the ambiguity set is
\[
\mathcal U_\rho
=
\left\{
Q:
D_{\mathrm{TV}}(Q\|\widehat P_{\mathrm{cal}}^S)\leq \rho
\right\},
\]
where
\[
D_{\mathrm{TV}}(Q\|P)
=
2\sup_A |Q(A)-P(A)|.
\]
The parameter \(\rho\) is the robustness budget. It controls how much the future score distribution is allowed to differ from the calibration score distribution. A larger \(\rho\) gives a wider voltage band and a more conservative screening decision.

For total variation, the robustification has a simple quantile interpretation. The usual conformal quantile level \(1-\alpha\) is replaced by
\[
\beta_{\alpha,\rho}^{\mathrm{TV}}
=
\min\left\{
1,\;
1-\alpha+\frac{\rho}{2}
\right\}.
\]
Thus, DR-CSS uses a higher quantile of the same calibration scores:
\[
\tau_\alpha^{\mathrm{rob}}(\rho)
=
s_{(k_{\alpha,\rho}^{\mathrm{TV}})},
\qquad
k_{\alpha,\rho}^{\mathrm{TV}}
=
\min\left\{
n_{\mathrm{cal}},
\left\lceil
(n_{\mathrm{cal}}+1)\beta_{\alpha,\rho}^{\mathrm{TV}}
\right\rceil
\right\}.
\]
This is the key practical rule: protecting against distribution shift is implemented by moving to a larger historical error quantile.

The robustness budget is selected using an independent tuning set generated
under the candidate controller configuration. For a given value of \(\rho\),
the empirical tuning coverage is
\begin{equation}
\hat c_{\mathrm{tun}}(\rho)
=
\frac{1}{n_{\mathrm{tun}}}
\sum_{m=1}^{n_{\mathrm{tun}}}
\mathbf{1}
\left\{
s_m^{\mathrm{new}}
\leq
\tau_{\alpha}^{\mathrm{rob}}(\rho)
\right\}.
\label{eq:appendix_tuning_coverage}
\end{equation}
Because this quantity is estimated from finitely many tuning scenarios, we use
the one-sided Wilson lower confidence bound
\begin{align}
L_{\delta_{\mathrm{tun}}}(\rho)
&:=
\mathrm{WLB}
\left(
\hat c_{\mathrm{tun}}(\rho),
n_{\mathrm{tun}},
\delta_{\mathrm{tun}}
\right),
\notag\\
\mathrm{WLB}(\hat c,n,\delta)
&:=
\max\left\{
0,\,
\frac{
\hat c+\frac{a}{2}
-
z\sqrt{\frac{\hat c(1-\hat c)+\frac{a}{4}}{n}}
}{
1+a
}
\right\},
\label{eq:appendix_wilson_bound}
\end{align}
where \(z=\Phi^{-1}(1-\delta)\) and \(a=z^2/n\). The selected robustness
budget is
\begin{equation}
\rho^\star
=
\inf
\left\{
\rho\geq 0:
L_{\delta_{\mathrm{tun}}}(\rho)
\geq
1-\alpha
\right\}.
\label{eq:appendix_rho_selection}
\end{equation}
Thus, DR-CSS selects the smallest robustness budget whose conservative
tuning-coverage estimate reaches the target level. If no admissible value
satisfies this condition, the available data do not support accepting the
candidate controller configuration.

The final robust band is not a deterministic proof of safety for all possible grid conditions. It is a statistical screening layer. It accepts a scenario only when the nominal trajectory, enlarged by a calibrated and robust error margin, remains within the voltage limits. Otherwise, it issues a warning because the simulator and available data are not sufficient to justify acceptance for that scenario.

\subsection{Predictor}

We use a sequence-to-sequence LSTM predictor to map the past grid-state window $\mathbf{x}_{1:H}$ to a multi-step voltage forecast
\[
    \hat V_{H+1:T}=\hat T(\mathbf{x}_{1:H}),
\]
for all $K$ monitored agents. The CP framework is model-agnostic; the LSTM can therefore be replaced by any predictor that provides multi-step voltage forecasts.

The predictor is trained on $N_{\mathrm{train}}$ trajectories by minimizing
\begin{equation}
    \min \sum_{i=1}^{N_{\mathrm{train}}}
    \sum_{t=H+1}^{T}
    \sum_{k=1}^{K}
    \bigl(V_{k,t}^{(i)}-\hat V_{k,t}^{(i)}\bigr)^2 .
\end{equation}
Training uses gradient-based optimization with a separate validation set for model selection. In the MA-COPP pipeline, the forecasts are used only to compute trajectory-level nonconformity scores for conformal calibration.
A grid search over the hyperparameters has been conducted. Table \ref{tab:gridsearch} summarizes the parameter ranges and the final selected hyperparameters. 
\begin{table}[h]
\centering
\caption{Predictor hyperparameter search. Selected values are highlighted.}
\label{tab:gridsearch}
\begin{tabular}{lll}
\toprule
Parameter & Tested values & Selected \\
\midrule
Hidden dimension & 64, 128, 256 & \textbf{128} \\
Layers & 1, 2 & \textbf{2} \\
Learning rate & $10^{-3}$, $2\times10^{-4}$ & $\mathbf{2\times10^{-4}}$ \\
Dropout & 0.0, 0.1 & \textbf{0.0} \\
Weight decay & 0.0, $10^{-5}$ & $\mathbf{10^{-5}}$ \\
Teacher forcing & 0.3, 0.5 & \textbf{0.5} \\
\bottomrule
\end{tabular}
\end{table}

The selected predictor achieves an MAE of $1.748\times10^{-3}$~p.u. and an RMSE of $3.066\times10^{-3}$~p.u. over the 10-step horizon, with a maximum observed error of $5.514\times10^{-2}$~p.u. The horizon-wise MAE increases from $7.34\times10^{-4}$~p.u. at $H+1$ to $2.327\times10^{-3}$~p.u. at $H+10$, reflecting the expected accumulation of uncertainty in multi-step forecasting.

\subsection{Extra Results}
This appendix provides supplementary IEEE 33-bus visual results that are not needed for the main comparison but help illustrate the behavior of the proposed screening layer on the smaller feeder. Fig.~\ref{fig:IEEE33_robustness_radius} shows the robustness-radius sweep, including the trade-off between empirical coverage and average band width. Fig.~\ref{fig:IEEE33_cp_interval} shows an example voltage trajectory with the corresponding conformal voltage band.

\input{figures/results_ieee33/robust_rho_plot_33}

\input{figures/results_ieee33/voltage_plot_33}

\input{figures/results_ieee141/robust_rho_plot}


We further examine the effect of the robustness radius \(\rho\) on the IEEE 141-bus system. As shown in Fig.~\ref{fig:ieee141-rho-sweep}, increasing \(\rho\) improves empirical coverage and eventually exceeds the nominal \(95\%\) level, but also increases the average width of the prediction regions. This confirms the expected coverage-conservativeness trade-off: larger $\rho$ provides stronger protection against policy-induced distribution shift at the cost of wider voltage bands. Fig.~\ref{fig:ieee141-voltage-example} illustrates this effect for a representative voltage trajectory, where the conformal region surrounds the nominal prediction over the forecast horizon and contains the realized future voltage.
