# Supplementary material for: Safety Screening for Voltage Control in Active Distribution Grids via Distributionally Robust Conformal Screening
Source: arXiv:2608.30889 source file (2026-08-31)
Supplement: Supplementary file 2 [file 07_Appendix_new.tex]

\section{Positioning Relative to Related Assurance Methods}
\label{app:positioning}

Table~\ref{tab:positioning} provides a qualitative positioning of DR-CSS relative to related assurance approaches. The comparison is intended to clarify the scope of the proposed method rather than rank the methods. The selected columns highlight the combination of properties targeted by DR-CSS: feeder-level voltage control, coverage guarantees, robustness to distribution shift, validation of learning-based control policies, and scenario-level accept/warning decisions.

% NOTE: 02_related_work_table.tex still says "DR-CSL" in the caption and in
% the final row. Fix both to "DR-CSS" in that file.
\input{02_related_work_table}


\subsection{Details on the Robust Statistical Abstraction}
\label{app:robust_calibration_details}

This appendix provides additional explanation of the robust conformal step used in DR-CSS, and is written to be self-contained: the quantities introduced in the main text are restated here in the form in which they are used. The goal is to clarify how the nominal simulator is converted into a statistical safety band.

For a scenario \(x\), the simulator returns a single trajectory \(\hat v_{H+1:T}=\Phi_M(x)\). If this trajectory is treated as exact, then the predictive distribution is the point mass \(P_x^{\mathrm{nom}}=\delta_{\hat v_{H+1:T}}\). This means that the simulator assigns probability one to the simulated trajectory and probability zero to all other possible futures. Such a representation is too confident for power-system validation, because the real trajectory may differ from the simulated one due to model mismatch, forecast error, topology uncertainty, measurement error, controller delay, or unmodeled dynamics.

DR-CSS therefore models the simulation error rather than trusting the simulated trajectory directly. For each calibration case \(j\), the scalar nonconformity score is
\begin{equation}
s_j
=
\max_{t\in\mathcal T_f}\max_{i\in\mathcal B}
\;\gamma_t\,
\frac{\bigl|V_{i,t}^{j}-\hat V_{i,t}^{j}\bigr|}
     {\hat\sigma_i^{\mathrm{err}}},
\label{eq:app_score}
\end{equation}
where \(V_{i,t}^{j}\) is the realized and \(\hat V_{i,t}^{j}\) the nominal simulated voltage magnitude at bus \(i\) and time \(t\), \(\hat\sigma_i^{\mathrm{err}}>0\) is the fixed bus-specific residual scale, and \(\gamma_t>0\) the fixed time weight. Thus \(s_j\) records the worst standardized voltage-prediction error over the whole horizon, reducing a high-dimensional trajectory error to one safety-relevant, dimensionless number. The empirical distribution
\[
\widehat P_{\mathrm{cal}}^S
=
\frac{1}{n_{\mathrm{cal}}}
\sum_{j=1}^{n_{\mathrm{cal}}}\delta_{s_j}
\]
is therefore a histogram of past worst-case simulation errors.

Standard conformal calibration uses a high quantile of this histogram. For \(\alpha=0.05\), this is approximately the 95\% quantile of the historical worst-case errors. The resulting band is valid when future errors are statistically similar to calibration errors. In conformal prediction, this similarity condition is called exchangeability. In the present setting, it means that future simulation-to-real voltage errors should behave like the historical errors used for calibration.

Control policy replacement may violate this condition. Historical data may come from a baseline control policy, while the tested deployment uses a new candidate policy. The new policy can move the system into different operating regions and change the simulation-error distribution. DR-CSS accounts for this by considering plausible post-deployment score distributions in a neighbourhood of the baseline score distribution.

Let \(P^{S}\) denote the population law of the score under baseline operation, of which \(\widehat P_{\mathrm{cal}}^S\) is the empirical counterpart, and let \(Q\) denote a candidate post-deployment law. Using total variation, the ambiguity set is
\begin{equation}
\mathcal U_\rho
=
\left\{
Q:
D_{\mathrm{TV}}\!\left(Q\,\|\,P^{S}\right)\leq \rho
\right\},
\qquad
D_{\mathrm{TV}}(Q\|P)
=
2\sup_A |Q(A)-P(A)| \in [0,2].
\label{eq:app_ambiguity}
\end{equation}
% NOTE: replace the citation key below with the one used for Cauchois et al.
% (Robust validation: confident predictions even when distributions shift)
% in your .bib file. If the key is wrong this prints [?].
We adopt the convention \(D_{\mathrm{TV}}\in[0,2]\) of~\cite{Cauchois2024RobustValidation}, which is the origin of the factor \(\rho/2\) in the inflated quantile level below. The empirical measure \(\widehat P_{\mathrm{cal}}^S\) enters only through the finite-sample order statistic. The parameter \(\rho\) is the robustness budget: it controls how much the post-deployment score distribution is allowed to differ from the baseline one. A larger \(\rho\) gives a wider voltage band and a more conservative screening decision.

For total variation, the robustification has a simple quantile interpretation. The usual conformal quantile level \(1-\alpha\) is replaced by
\begin{equation}
\beta_{\alpha,\rho}^{\mathrm{TV}}
=
\min\left\{
1,\;
1-\alpha+\frac{\rho}{2}
\right\},
\label{eq:app_beta_tv}
\end{equation}
so that DR-CSS uses a higher quantile of the same calibration scores,
\begin{equation}
\tau_\alpha^{\mathrm{rob}}(\rho)
=
s_{(k_{\alpha,\rho}^{\mathrm{TV}})},
\qquad
k_{\alpha,\rho}^{\mathrm{TV}}
=
\min\left\{
n_{\mathrm{cal}},
\left\lceil
(n_{\mathrm{cal}}+1)\,\beta_{\alpha,\rho}^{\mathrm{TV}}
\right\rceil
\right\},
\label{eq:app_tau_rob}
\end{equation}
where \(s_{(k)}\) is the \(k\)-th smallest calibration score. This is the key practical rule: protecting against distribution shift is implemented by moving to a larger historical error quantile.

The robustness budget is selected using an independent tuning set generated under the candidate joint policy \(\pi^{\mathrm{dep}}\). For a given value of \(\rho\), the empirical tuning coverage is
\begin{equation}
\hat c_{\mathrm{tun}}(\rho)
=
\frac{1}{n_{\mathrm{tun}}}
\sum_{m=1}^{n_{\mathrm{tun}}}
\mathbf{1}
\left\{
s_m^{\mathrm{new}}
\leq
\tau_{\alpha}^{\mathrm{rob}}(\rho)
\right\},
\label{eq:app_tuning_coverage}
\end{equation}
with \(s_m^{\mathrm{new}}\) computed from~\eqref{eq:app_score} using the same fixed \(\hat\sigma_i^{\mathrm{err}}\) and \(\gamma_t\). Because this quantity is estimated from finitely many tuning scenarios, we use the one-sided Wilson lower confidence bound
\begin{align}
L_{\delta_{\mathrm{tun}}}(\rho)
&:=
\mathrm{WLB}
\left(
\hat c_{\mathrm{tun}}(\rho),\,
n_{\mathrm{tun}},\,
\delta_{\mathrm{tun}}
\right),
\notag\\[4pt]
\mathrm{WLB}(\hat c,n,\delta)
&:=
\max\left\{
0,\;
\frac{
\hat c+\dfrac{a}{2}
-
z\sqrt{\dfrac{\hat c(1-\hat c)}{n}+\dfrac{a}{4n}}
}{
1+a
}
\right\},
\label{eq:app_wilson_bound}
\end{align}
where \(z=\Phi^{-1}(1-\delta)\), \(a=z^2/n\), and \(\Phi\) is the standard normal cumulative distribution function. The selected robustness budget is
\begin{equation}
\rho^\star
=
\inf
\left\{
\rho\geq 0:
L_{\delta_{\mathrm{tun}}}(\rho)
\geq
1-\alpha
\right\}.
\label{eq:app_rho_selection}
\end{equation}
Thus, DR-CSS selects the smallest robustness budget whose conservative tuning-coverage estimate reaches the target level. If no admissible value satisfies this condition, the available data do not support accepting the candidate policy configuration.

\paragraph*{Origin of the tuning data}
The tuning scores \(s_m^{\mathrm{new}}\) in~\eqref{eq:app_tuning_coverage} require realized trajectories under \(\pi^{\mathrm{dep}}\). In our experiments these are produced by the high-fidelity environment, which plays the role of the physical grid. In practice, an operator can obtain them from (i) a limited pilot deployment restricted to a safe operating envelope, (ii) an independent higher-fidelity model or hardware-in-the-loop setup distinct from \(\Phi_M\), or (iii) the intermediate stages of the gradual replacement strategy, in which each deployment stage supplies tuning data for the next. When no such data exist, \(\rho\) must be fixed a priori from engineering judgement, and the tuning-coverage bound~\eqref{eq:app_wilson_bound} does not apply.

\paragraph*{Scope of the guarantee}
Under exchangeability of the calibration scores, and provided the post-deployment score law lies in \(\mathcal U_{\rho^\star}\), the robust band attains coverage at least \(1-\alpha\) for the post-deployment voltage trajectory, jointly over all buses and future time steps. Equivalently, the screening rule controls the probability of accepting an unsafe scenario,
\begin{equation}
\Pr\left[\,\mathrm{accept}(x)\;\wedge\;g(v_{H+1:T})>0\,\right]\leq\alpha .
\label{eq:app_safety_claim}
\end{equation}
We emphasise that \(\rho^\star\) is itself selected from tuning data via~\eqref{eq:app_rho_selection}. The Wilson bound controls the selection error at level \(\delta_{\mathrm{tun}}\) for each fixed \(\rho\), and we do not claim uniform validity along the selection path. The final robust band is therefore not a deterministic proof of safety for all possible grid conditions; it is a calibrated statistical screening layer. It accepts a scenario only when the nominal trajectory, enlarged by a calibrated and robust error margin, remains within the voltage limits. Otherwise, it issues a warning, because the simulator and available data are not sufficient to justify acceptance for that scenario.


\subsection{Nominal Simulator: Implementation and Rationale}
\label{app:predictor}

In our experiments the nominal simulator \(\Phi_M\) is realized by a sequence-to-sequence LSTM predictor mapping the past grid-state window \(\mathbf{x}_{1:H}\) to a multi-step voltage forecast
\begin{equation}
    \hat V_{H+1:T}=\hat T(\mathbf{x}_{1:H}),
\label{eq:app_predictor}
\end{equation}
for all \(K=|\mathcal B|\) monitored buses.

This choice deserves comment. In the problem formulation, \(\Phi_M\) is defined as a closed-loop rollout taking the deployed policy \(\pi^{\mathrm{dep}}\) as an argument, whereas \(\hat T\) conditions on the observed history only. The restriction is deliberate. DR-CSS is motivated by the fact that distribution-grid operators rarely possess a simulator that is simultaneously accurate, fully observable, and policy-aware: models suffer from incomplete observability, imperfect topology knowledge, and unmodelled device interactions. A closed-loop rollout with exact knowledge of \(\pi^{\mathrm{dep}}\) would not reproduce these conditions, and screening against such a simulator would understate the simulation-to-reality gap that DR-CSS is designed to absorb.

We therefore use \(\hat T\) as a deliberately imperfect nominal model. Its approximation error stands in for the aggregate model deficiency an operator faces in practice, and the resulting discrepancy is captured through the nonconformity scores rather than modelled explicitly. Both shift components consequently enter through the score distribution: the simulation-to-reality shift through the predictor's approximation error, and the policy-induced shift through the change in operating conditions that \(\hat T\) cannot anticipate. The robust enlargement in~\eqref{eq:app_tau_rob} is what covers the latter.

The framework itself is agnostic to this choice. A policy-conditioned \(\Phi_M\) --- an AC power-flow rollout, a reduced-order model, or a learned closed-loop surrogate --- can be substituted without modification, and would be expected to reduce the required robustness budget \(\rho^\star\) by moving part of the policy-induced shift out of the residual and into the prediction. The reported values of \(\rho^\star\) should therefore be read as an upper range, obtained under a nominal model unaware of the candidate policy.

The predictor is trained on \(N_{\mathrm{train}}\) trajectories by minimizing
\begin{equation}
    \min \sum_{i=1}^{N_{\mathrm{train}}}
    \sum_{t=H+1}^{T}
    \sum_{k=1}^{K}
    \bigl(V_{k,t}^{(i)}-\hat V_{k,t}^{(i)}\bigr)^2 .
\label{eq:app_training_loss}
\end{equation}
Training uses gradient-based optimization with a separate validation set for model selection. The bus-specific residual scales \(\hat\sigma_i^{\mathrm{err}}\) used in~\eqref{eq:app_score} are estimated on this same validation split and held fixed thereafter, so that they are independent of the calibration, tuning, and test scores. The forecasts enter DR-CSS only through the trajectory-level nonconformity scores; the same forecasts are used for all compared methods, so the reported differences reflect the calibration procedure rather than predictor quality.

A grid search over the hyperparameters has been conducted. Table~\ref{tab:gridsearch} summarizes the parameter ranges and the final selected hyperparameters.
\begin{table}[h]
\centering
\caption{Predictor hyperparameter search. Selected values are highlighted.}
\label{tab:gridsearch}
\begin{tabular}{lll}
\toprule
Parameter & Tested values & Selected \\
\midrule
Hidden dimension & 64, 128, 256 & \textbf{128} \\
Layers & 1, 2 & \textbf{2} \\
Learning rate & $10^{-3}$, $2\times10^{-4}$ & $\mathbf{2\times10^{-4}}$ \\
Dropout & 0.0, 0.1 & \textbf{0.0} \\
Weight decay & 0.0, $10^{-5}$ & $\mathbf{10^{-5}}$ \\
Teacher forcing & 0.3, 0.5 & \textbf{0.5} \\
\bottomrule
\end{tabular}
\end{table}

The selected predictor achieves an MAE of \(1.748\times10^{-3}\)~p.u.\ and an RMSE of \(3.066\times10^{-3}\)~p.u.\ over the 10-step horizon, with a maximum observed error of \(5.514\times10^{-2}\)~p.u. The horizon-wise MAE increases from \(7.34\times10^{-4}\)~p.u.\ at \(H+1\) to \(2.327\times10^{-3}\)~p.u.\ at \(H+10\), reflecting the expected accumulation of uncertainty in multi-step forecasting.
% NOTE: verify the source of the 5.514e-2 outlier before keeping the
% sentence below; adapt or delete if the cause is different.
The maximum error is comparable to half the admissible voltage band and arises in a small number of scenarios with rapid changes in net injection at the feeder ends. Such outliers are precisely what the upper tail of the calibration score distribution is intended to capture, and they motivate the trajectory-level maximum in~\eqref{eq:app_score} rather than an averaged error measure.


\subsection{Extra Results}
\label{app:extra_results}

This appendix provides supplementary visual results that are not needed for the main comparison but help illustrate the behavior of the proposed screening layer. Fig.~\ref{fig:IEEE33_robustness_radius} shows the robustness-radius sweep for the IEEE 33-bus system, including the trade-off between empirical coverage and average band width, and Fig.~\ref{fig:IEEE33_cp_interval} shows an example voltage trajectory with the corresponding conformal voltage interval on the same feeder.

\input{figures/results_ieee33/robust_rho_plot_33}

\input{figures/results_ieee33/voltage_plot_33}

\input{figures/results_ieee141/robust_rho_plot}

We further examine the effect of the robustness radius \(\rho\) on the IEEE 141-bus system. As shown in Fig.~\ref{fig:ieee141-rho-sweep}, increasing \(\rho\) improves empirical coverage and eventually exceeds the nominal \(95\%\) level, but also increases the average width of the prediction intervals. This confirms the expected coverage--conservativeness trade-off: larger \(\rho\) provides stronger protection against policy-induced distribution shift at the cost of wider voltage bands. The sweep also shows that the selected \(\rho^\star\) lies in the region where coverage first reaches the target, consistent with the selection rule~\eqref{eq:app_rho_selection}.
